# Supplementary material for: Online Market Equilibrium with Application to Fair Division
Source: arXiv:2103.12936 source file (2021-10-02)
Supplement: Supplementary file 1 [file appendix.tex]

\section*{Appendix}
	\subsection*{Proof of Theorem \ref{thm:asymp-envy-free}}
    \begin{proof}
        By the definition of $\bar{x}^t_i$, we have 
        \[ \langle v_i, \bar{x}^t_i\rangle = \frac{1}{t} \sum_{\tau=1}^t v_{ij_\tau}\ind\{i=i_\tau\} = \bar{g}^t_i. \]
        Let $p^*_j = \max_i \beta^*_i v_{ij}$ be the equilibrium prices. We have, for any $i$,
        \begin{align}
            \langle p^*, \bar{x}^t_i \rangle &= \frac{1}{t}\sum_{\tau=1}^t p^*_{j_\tau} \ind\{ i = i_\tau \} \nonumber \\
            & = \bar{b}^t_i + \frac{1}{t}\sum_{\tau=1}^t (p^*_{j_\tau} -\beta^\tau_i v_{ij_\tau})\ind\{ i=i_\tau \} \nonumber \\
            & \leq B_i + \Delta^t_i + \eta^t_i, \label{eq:bounding-p*-x(i,t)}
            % & = B_i + O\left( \frac{(\log t)^2}{t} \right).
        \end{align}
        
        Furthermore, note that, for any $k \neq i$, 
        \[ \left \langle p^*, \frac{B_i}{B_k} \bar{x}^t_k \right\rangle \leq \frac{B_i}{B_k}(B_k+\Delta^t_k+\eta^t_k) =  B_i \left(1 + \frac{\Delta^t_k+\eta^t_k}{B_k} \right). \]
         Since $x^*_i \in D_i(p^*)$, we have (recall that $u^*_i \leq 1$ by Lemma \ref{lemma:bounds-on-beta})
        \[ \left \langle v_i, \frac{B_i}{B_k} \bar{x}^t_k \right \rangle \leq u^*_i \left(1 + \frac{\Delta^t_k+\eta^t_k}{B_k} \right) \leq u^*_i + \frac{\Delta^t_k+\eta^t_k}{B_k} \leq \langle v_i, \bar{x}^t_i\rangle + \xi^t_i + \frac{\Delta^t_k+\eta^t_k}{B_k}. \]
        Hence,
        \begin{align}
            & \frac{\langle v_i, \bar{x}^t_k\rangle}{B_k} \leq \frac{\langle v_i, \bar{x}^t_i\rangle}{B_i} + \frac{\xi^t_i}{B_i} + \frac{ \Delta^t_k+\eta^t_k }{B_i B_k} \nonumber \\
            \Rightarrow \ &\rho^t_i \leq \frac{\xi^t_i}{B_i} + \frac{1}{B_i} \max_k \frac{ \Delta^t_k+\eta^t_k }{B_k} \leq \kappa \xi^t_i + \kappa^2\max_k (\Delta^t_k+\eta^t_k). \label{eq:rho(t,i)<=...}
        \end{align}
        
        % The bounds on $\EE (\xi^t_i)^2$ and $\EE (\Delta^t_i)^2$ used in the theorem are given by Theorems~\ref{thm:conv-utilities} and~\ref{thm:conv-expenditures}, respectively. %It remains to bound $\EE (\eta^t_i)^2$.
        
        To establish the convergence of $\eta^t_i$, by \eqref{eq:bound-|p*(j)-max-beta(i,t)*v(i,j)|-any-j},
        % \ck{I removed subscript $i$ from $\|v_i\|_\infty$ in the last expression, please check. Something was weird with $i$ subscripts below I think. Please use $i$ and $i'$ or something, for different meanings. I removed more $i$ subscripts from inf norms below} \yuan{Yes you are right. There shouldn't be subscripts.} 
            \begin{align}
                |\eta^t_i| \leq \sum_\ell |\eta^t_\ell| \leq \frac{1}{t}\sum_{\tau=1}^t |p^*_{j_\tau} -\beta^\tau_{i_\tau} v_{i_\tau j_\tau} | \leq \frac{1}{t}\sum_{\tau=1}^t \|v\|_\infty \|\beta^\tau - \beta^*\|_\infty = \gamma_t.
                % \leq \|v\|_\infty\frac{1}{t}\sum_{\tau=1}^t \|\beta^\tau - \beta^*\|. 
                \label{eq:bound-eta(t,i)}
            \end{align}
        Hence, same as \eqref{eq:bound-gamma(t)},
            \begin{align}
                \EE (\eta^t_i)^2 \leq \|v\|_\infty^2 \frac{1}{t}\sum_{\tau=1}^t \EE \|\beta^\tau - \beta^*\|^2 \leq \|v\|_\infty^2 \frac{1}{t} \left( 6(1+\log t) + \frac{(\log t)^2}{2} \right) \frac{G^2}{\sigma^2}. \label{eq:bound-E(eta(t,i))}
            \end{align}
            By Theorems~\ref{thm:conv-beta(t)} and~\ref{thm:conv-expenditures}, we know that $\EE (\xi^t_i)^2 = O\left(\frac{\log t}{t}\right)$ and $\EE(\Delta^t_i)^2 = O\left(\frac{(\log t)^2}{t}\right)$. Together with \eqref{eq:bound-E(eta(t,i))} and \eqref{eq:rho(t,i)<=...}, we deduce
            \[ \EE(\rho^t_i)^2 \leq \kappa \EE(\xi^t_i)^2 + \kappa^2 \sum_\ell (\EE (\Delta^t_\ell)^2 + \EE(\eta^t_\ell)^2) = O\left(\frac{(\log t)^2}{t}\right). \]
        \end{proof}
